# Supplementary material for: In-House Evaluation Is Not Enough: Towards Robust Third-Party Flaw Disclosure for General-Purpose AI
Source: arXiv:2503.16861 source file (2025-03-25)
Supplement: Supplementary file 1 [file 99_appendix.tex]

\tableofcontents
\clearpage

\section{Terminology \& Definitions}\label{app:definitions}

\subsection{Key Definitions}

In \Cref{fig:definitions} we outline key definitions for terms used in this work, along with their justifications.

\input{tables/definitions}

\input{sections/9.1_related_definitions}

\input{sections/9.2_diff_incident_flaw}

\input{sections/8_flaw_report_details}

\section{Policy Recommendations and Details}\label{app:policy}

\subsection{Recommendations for Policymakers}

\input{sections/6_policy}

\input{sections/6_policy_overview}

\input{sections/6_policy_safe_harbors}

\input{sections/6_policy_illegal_flaws}

\input{sections/7_risk_taxonomy}
